# Supplementary material for: Scattering Statistics in Nonlinear Wave Chaotic Systems
Source: arXiv:1812.06789 ancillary file (2018-12-13)
Supplement: Supplementary file 1 [file supplemental.pdf]

# (supplemental) Scattering Statistics in Nonlinear Wave Chaotic Systems

Min Zhou,[1,2] Edward Ott,[1,3] Thomas M. Antonsen, Jr,[1,3] and Steven M. Anlage[1,2,3]

[1]*Department of Electrical and Computer Engineering, University of Maryland, College Park, Maryland 20742, USA*
[2]*Center for Nanophysics and Advanced Materials, University of Maryland, College Park, Maryland 20742, USA*
[3]*Department of Physics, University of Maryland, College Park, Maryland 20742, USA*

(Dated: December 13, 2018)

In this document we provide supplemental information on the high-power vector network analyzer (VNA), as well as simulations of the diode-loaded port in computer simulation technology (CST).

## I. HIGH POWER VNA

The Vector Network Analyzer (Keysight N5242A PNA-X) has been upgraded with high power option H85 [1]. By removing the bias tee, it enables fully calibrated high power S-parameters measurements up to 20 W (+43 dBm). The external booster amplifier, coupler, attenuator, and isolators are chosen as follows. We have used an RF-Lambda amplifier RFLUPA0218G5 working in the frequency range of 2-18 GHz, with output power up to +38 dBm (3 dB compression). By adding couplers (RF-Lambda RFDC2G18G20) and additional attenuators, this configuration is optimized for high power measurement. Note that the signal to noise ratio (SNR) is decreased as the excitation power decreases. Measurements are taken at powers of -5, +5, +15, +25, and +30 dBm, in the frequency range 4 $\sim$ 18 GHz, limited by the isolator (Fairview Microwave SFI0418) bandwidth.

## II. SIMULATION IN CST

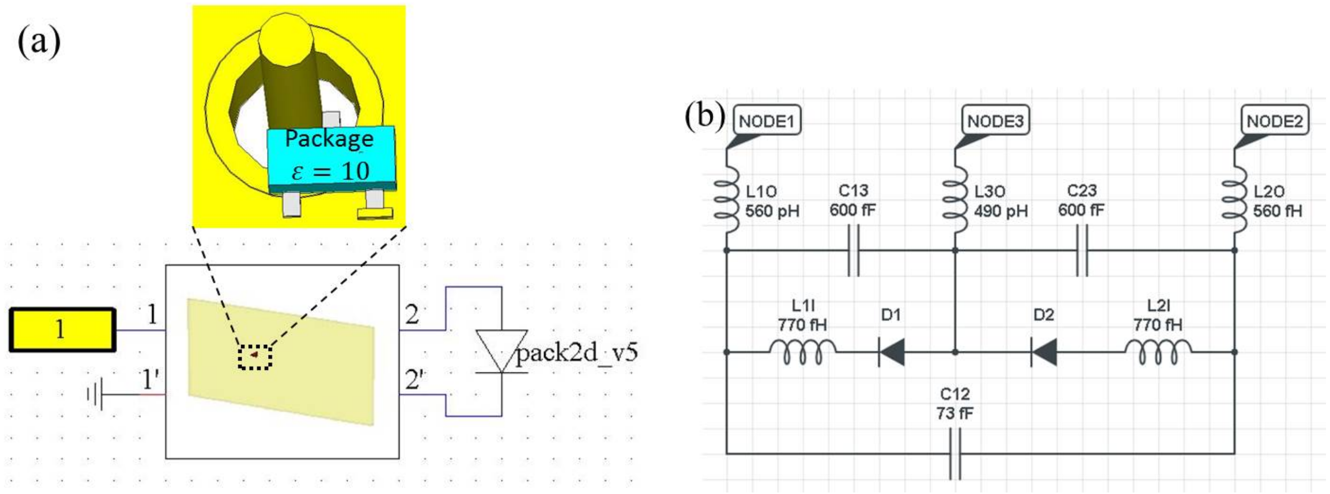


FIG. S1. (a) Model in CST to simulate the radiation S-parameters of the nonlinear port. The physical dimension and dielectric properties of the diode package are included in the CST model. Note that the parallel plate waveguide is terminated with radiating boundary conditions on all sides. (b) The complete SPICE model of the diode and the package, indicated as 'pack2d_v5' in (a).

To create a model that resembles the nonlinear port in CST, we first draw a 3D model that has the same dimensions as the physical port. All of the product information about the diode and its packaging can be found on the manufacturer's webpage [2]. We have taken into account the diode package dimensions, the SPICE model of the diode and the SPICE model of the package. Fig. S1(a) shows the port configuration in CST. The physical diode package is approximated as a dielectric block with its relative dielectric constant used as a fitting parameter (fitted $\epsilon_r = 10$ as shown in Fig. S1(a)). The radiation scattering parameter is a property of the port, hence the shape of the cavity does not play a role. In other words we establish a condition where the waves radiating from the port are not reflected back to the port. To achieve this, the top and bottom parallel rectangular plates are terminated with radiation boundary conditions. There is only one external excitation port which is defined on

the antenna, and it is labelled as the yellow block with number "1" in Fig. S1(a). To include the SPICE model of the diode and package, another differential port, port 2, is also built between the center pin and ground. The SPICE models of the diode and the package are integrated into one file "pack2d_v5" and attached to port 2. The details of the SPICE model are given in Fig. S1(b). There are two diodes in the package, and three pins, but we only connected two pins, say between node 3 and node 2. The package model is specified to be valid up to 6 GHz. To adapt the model to our situation where frequency is applied up to 18 GHz, we have adjusted all the parasitic capacitances, i.e. C13, C23, and C12, to be approximately 2 orders of magnitude smaller than specified. The diode model for D1 and D2 is the standard SPICE model including both DC characteristics and dynamic effects.

The results of the simulation are shown in Fig. S2(b), and compared with the radiation case experimental results shown in Fig. S2(a). The black curve is the radiation S-parameter for the linear case where there is no diode attached to the port. Adding the diode, the overall coupling to the cavity is changed substantially, and this is captured in the model. When changing the amplitude of the incident wave from 0.1 V to 10 V, the simulated radiation S-parameters show similar amplitude dependence as the experimental results. Thus the model captures the essential behavior of the nonlinear port radiation properties.

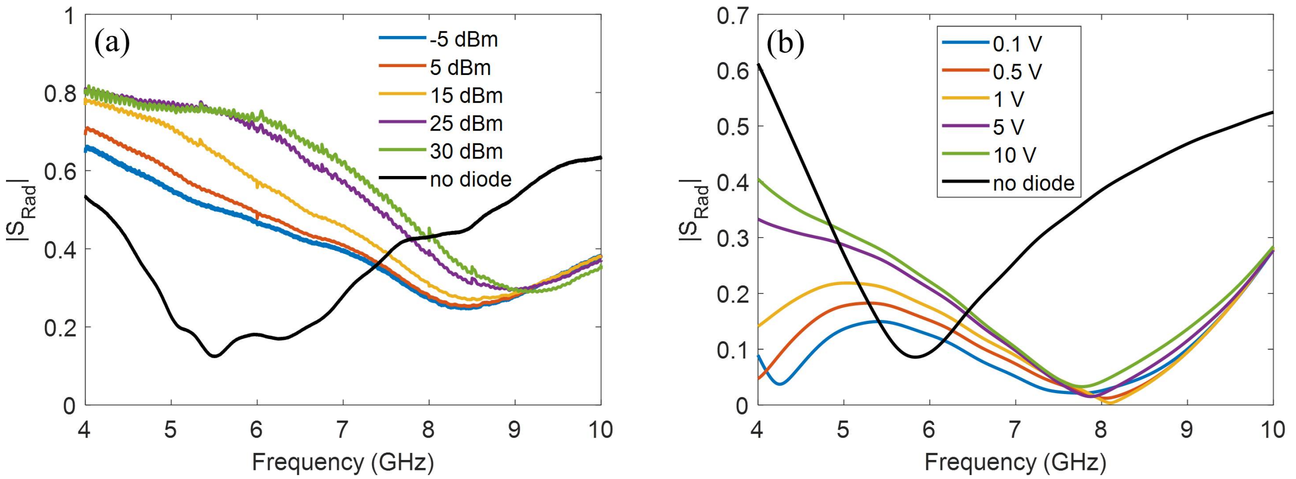


FIG. S2. (a) Experimental results of the radiation S-parameters at different input powers. (b) Simulation in CST by importing the SPICE model of the diode and package, and adding a dielectric block representing the physical dimension of the package. $|S_{Rad}|$ for different amplitudes with diode and no diode case.

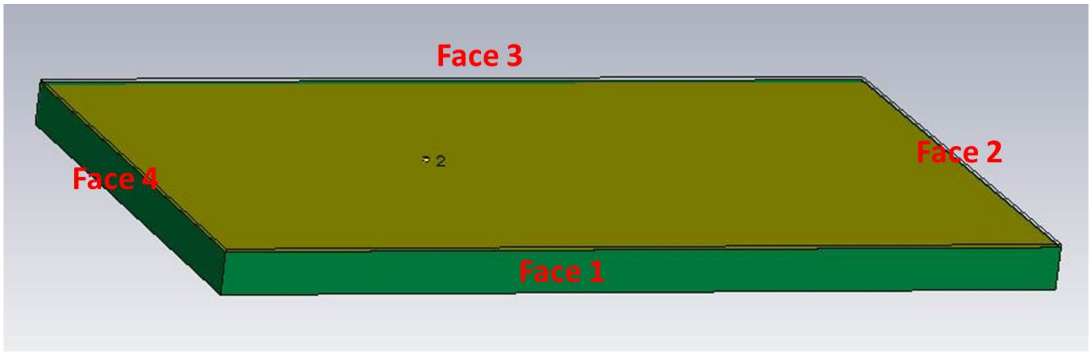


FIG. S3. Model in CST to simulate the radiation efficiency with the nonlinear port. Four faces are defined along the perimeter of the parallel plate structure, and the port is labelled '2'. The total power radiated through the boundary can be calculated by integrating the power density along each face, and summing them up along these 4 faces.

Furthermore, we are also able to simulate the port radiation efficiency, which is the ratio of the radiated power

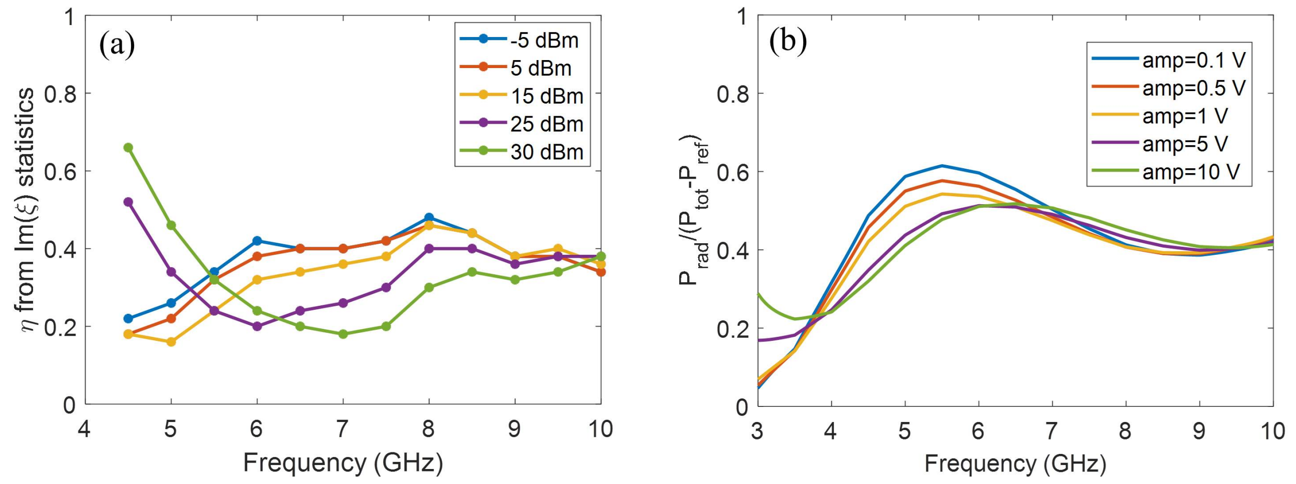


FIG. S4. (a) Experimental radiation efficiency obtained by fitting the statistics of $\xi$. (b) Radiation efficiency simulated in CST, by directly calculating the ratio of $P_{rad}/(P_{tot} - P_{ref})$.

to the input power at the port. The total power from the source $P_{tot}$ is decomposed into several parts, i.e. the power directly reflected by the port $P_{ref}$, the power loss at the port, the power loss in the cavity, and the power radiated through the boundary $P_{rad}$. The power loss by the cavity is the Ohmic loss of the copper parallel plate which is negligible. The input power at the port can be calculated from the difference between the total power $P_{tot}$ and the reflected power $P_{ref}$. In the simulation, the total power is a constant over frequency, and the reflected power can be calculated from the simulated $S_{11}$. To get the radiated power, we have defined 4 faces along the boundary of the parallel plate model, as shown in Fig. S3. By integrating power on these 4 faces and summing them up, we can get the total power radiated $P_{rad}$.

The radiation efficiency $\eta$ is then calculated as $\eta = P_{rad}/(P_{tot} - P_{ref})$. Fig. S4(b) shows the simulated radiation efficiency for different input amplitudes of the nonlinear port. Also shown are the experimental results in Fig. S4(a), where the radiation efficiency $\eta$ is fitted by comparing the statistics of normalized impedance $\xi$ with that in the linear case. It is clear that the CST simulation reproduces the key features of the experimental case. There is a regime in which $\eta$ increases with power at low frequency. In the intermediate frequency regime, the radiation efficiency decreases as the incident power increases. At high frequency, the behavior tends to be power independent. Therefore we conclude that the radiation efficiency model captures the essential behavior of the nonlinear port.

[1] keysight PNA high power user's guide: http://literature.cdn.keysight.com/litweb/pdf/N5242-90008.pdf
[2] Infineon BAS70-04 product information: https://www.infineon.com/cms/en/product/transistor-diode/diode/schottky-diode/high-speed-switching-clipping-and-clamping/bas70-04/
